# Supplementary material for: Formation of Organic Color Centers in Air-Suspended Carbon Nanotubes Using Vapor-Phase Reaction
Source: arXiv:2103.00689 ancillary file (2021-03-01)
Supplement: Supplementary file 1 [file SI_DopedSuspendedTubes.pdf]

# Supplementary Information for "Formation of Organic Color Centers in Air-Suspended Carbon Nanotubes Using Vapor-Phase Reaction"

Daichi Kozawa,[1,*] Xiaojian Wu,[2] Akihiro Ishii,[1,3]
Jacob Fortner,[2] Keigo Otsuka,[3] Rong Xiang,[4] Taiki Inoue,[4]
Shigeo Maruyama,[4] YuHuang Wang,[2,5] and Yuichiro K. Kato[1,3,†]

[1]*Quantum Optoelectronics Research Team,*
*RIKEN Center for Advanced Photonics, Saitama 351-0198, Japan*
[2]*Department of Chemistry and Biochemistry, University of Maryland,*
*College Park, Maryland 20742, United States*
[3]*Nanoscale Quantum Photonics Laboratory,*
*RIKEN Cluster for Pioneering Research, Saitama 351-0198, Japan*
[4]*Department of Mechanical Engineering,*
*The University of Tokyo, Tokyo 113-8656, Japan*
[5]*Maryland NanoCenter, University of Maryland,*
*College Park, Maryland 20742, United States*

[*] Corresponding author. daichi.kozawa@riken.jp
[†] Corresponding author. yuichiro.kato@riken.jp

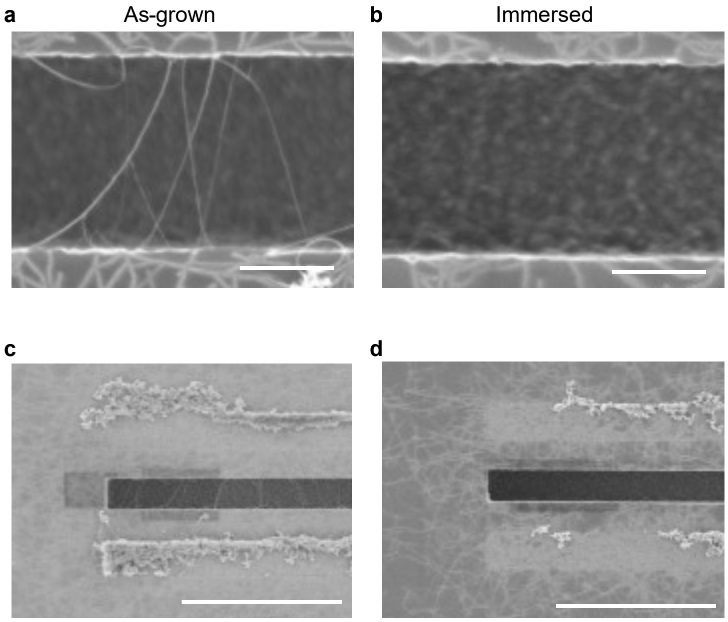


FIG. S1. Scanning electron micrographs of suspended SWCNTs across a trench with a width of 1.0 $\mu$m, which are taken in representative regions for (a) before and (b) after immersing the sample in water for 60 s and dried on a hot plate at 80 °C for 60 s. Panels (c) and (d) are zoomed-out images of trenches (c) before and (d) after the immersion, respectively. The scale bars in (a,b) and (c,d) are 500 nm and 5 $\mu$m, respectively.

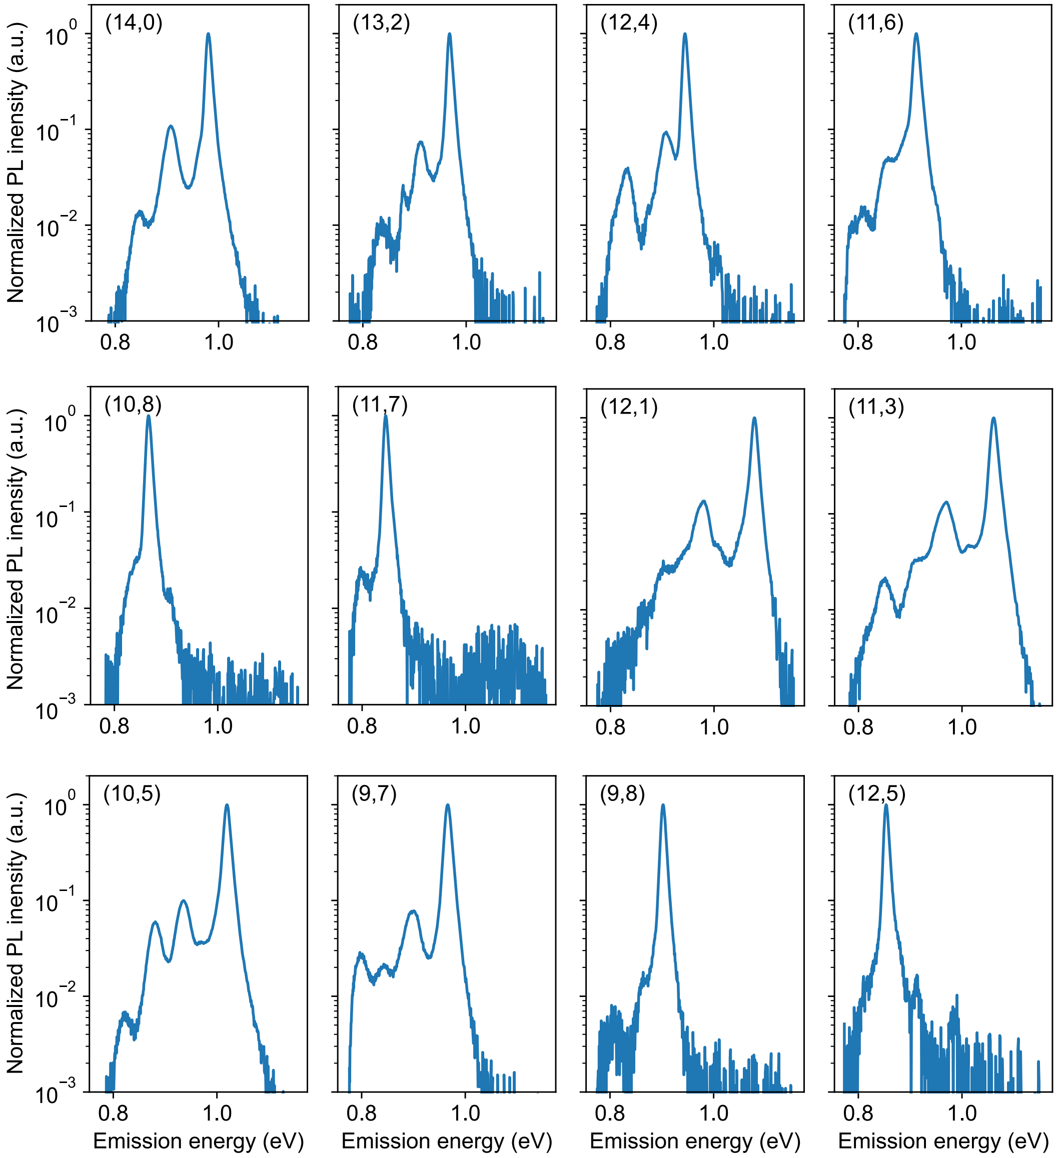


FIG. S2. Representative PL spectra of functionalized SWCNTs measured with the same excitation condition as Fig. 2, where the vertical axis is in a logarithmic scale.

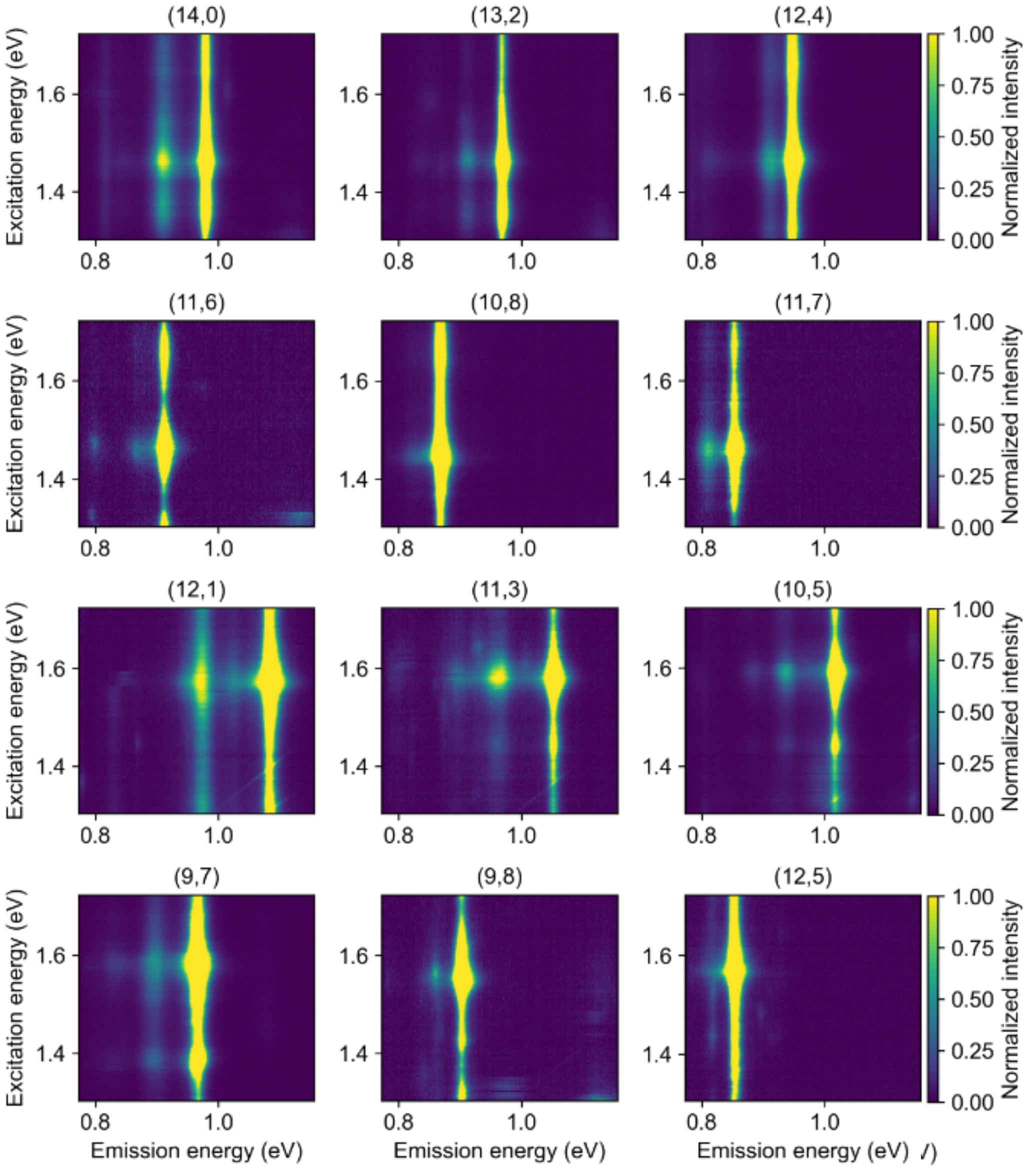


FIG. S3. PL excitation maps for various chiralities of functionalzied SWCNTs measured with an excitation power of 100 $\mu$W.

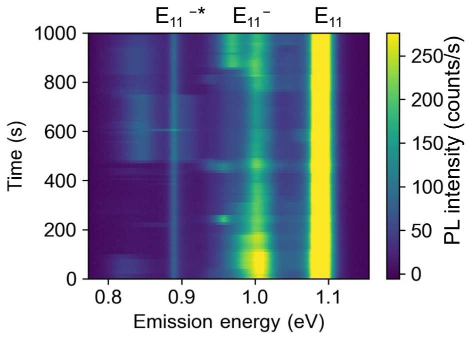


FIG. S4. A PL time trace of a functionalized (11,3) SWCNT exposed for 10 s each at the same spot over 1000 s, where the measurements are performed with an excitation energy of 1.59 eV and a power of 100 $\mu$W.

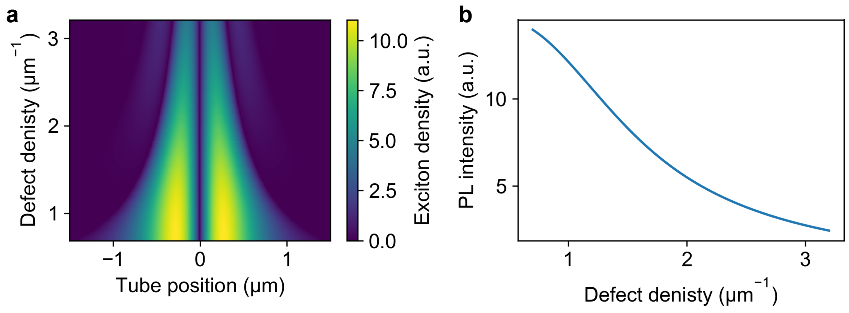


FIG. S5. Simulations of defect density dependence on (a) exciton density spatial profile and (b) PL intensity for a functionalized tube with a diameter of 1.00 nm.

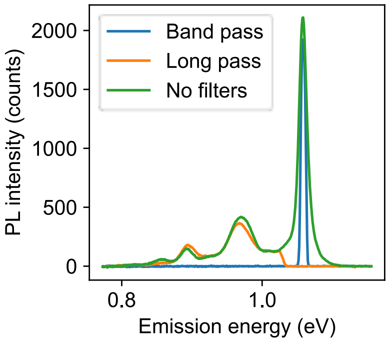


FIG. S6. PL spectra of a functionalized (11,3) SWCNT measured with a band-pass filter (blue) or a long-pass filter (orange) to differentiate $E_{11}$ emission from $E_{11}^{-}$ and $E_{11}^{-*}$ emission. A PL spectrum obtained without the filters is also shown in green.
